# Supplementary material for: Multi-resolution encoding and optimization for next generation video compression
Source: arXiv:2301.12191 source file (2023-01-28)
Supplement: Supplementary file 1 [file kth_appendix4_abr_results.tex]

\chapter{Detailed results of HEVC ABR streaming methods}
\label{sec:hevc_abr_res}

\begin{table}[!htbp]
\centering
\begin{tabular}{|p{2.8cm} | p{2.0cm} |p{2.5cm}| p{1.5cm}| p{1.5cm} |p{1.8cm} |}
\hline
\multicolumn{6}{|c|}{Test for CQP representations}\\
\hline
Video & Resolution & Analysis level &	$\Delta$T & BD-Rate & BD-PSNR\\
\hline
\rowcolor{blue!5} BasketBallDrive &	960x540 &	4 &	12.41 \% &	2.53 \% &	-0.11 dB \\
\rowcolor{gray!10} BasketBallDrive &	960x540 &	6 &	14.19 \% &	2.53 \% &	-0.11 dB \\
\rowcolor{blue!5} BasketBallDrive &	960x540 &	10 &	51.34 \% &	17.45 \% &	-0.64 dB \\
\rowcolor{gray!10} BasketBallDrive &	1920x1080 &	4 &	12.67 \% &	3.29 \% &	-0.08 dB \\
\rowcolor{blue!5} BasketBallDrive &	1920x1080 &	6 &	14.28 \% &	3.29 \% &	-0.08 dB \\
\rowcolor{gray!10} BasketBallDrive &	1920x1080 &	10 &	40.65 \% &	38.75 \% &	-0.60 dB \\
\rowcolor{blue!5} CrowdRun &	960x540 &	4 &	15.65 \% &	1.86 \% &	-0.08 dB \\
\rowcolor{gray!10} CrowdRun &	960x540 &	6 &	16.27 \% &	1.86 \% &	-0.08 dB \\
\rowcolor{blue!5} CrowdRun &	960x540 &   10 &	52.28 \% &	9.49 \% &	-0.39 dB \\
\rowcolor{gray!10} CrowdRun &	1920x1080 &	4 &	13.92 \% &	2.49 \% &	-0.10 dB \\
\rowcolor{blue!5} CrowdRun &	1920x1080 &	6 &	14.39 \% &	2.49 \% &	-0.10 dB \\
\rowcolor{gray!10} CrowdRun &	1920x1080 &	10 &	52.20 \% &	14.45 \% &	-0.48 dB \\
\rowcolor{blue!5} DucksTakeOff &	960x540 &	4 &	18.01 \% &	0.55 \% &	-0.02 dB \\
\rowcolor{gray!10} DucksTakeOff &	960x540 &	6 &	19.85 \% &	0.55 \% &	-0.02 dB \\
\rowcolor{blue!5} DucksTakeOff &	960x540 &	10 &	54.77 \% &	9.87 \% &	-0.34 dB \\
\rowcolor{gray!10} DucksTakeOff &	1920x1080 &	4 &	8.13 \% &	0.31 \% &	-0.01 dB \\
\rowcolor{blue!5} DucksTakeOff &	1920x1080 &	6 &	9.82 \% &	0.31 \% &	-0.01 dB \\
\rowcolor{gray!10} DucksTakeOff &	1920x1080 &	10 &	57.13 \% &	11.88 \% &	-0.34 dB \\
\hline
\textbf{Average} & \textbf{960x540} & \textbf{4} &	 \textbf{15.87 \% }  &	\textbf{1.65 \%} & \textbf{-0.07 dB } \\
\textbf{Average} & \textbf{960x540} & \textbf{6} &	\textbf{17.23 \% }   &  \textbf{1.65 \%} & \textbf{-0.07 dB } \\
\textbf{Average} & \textbf{960x540} & \textbf{10} & \textbf{53.06 \% }&	\textbf{12.27\%} & \textbf{-0.46 dB } \\
\hline
\textbf{Average} & \textbf{1920x1080} & \textbf{4} &	 \textbf{11.57 \% }  &	\textbf{2.03 \%} & \textbf{-0.06 dB } \\
\textbf{Average} & \textbf{1920x1080} & \textbf{6} &	\textbf{12.83 \% }   &  \textbf{2.03 \%} & \textbf{-0.06 dB } \\
\textbf{Average} & \textbf{1920x1080} & \textbf{10} & \textbf{49.99 \% }&	\textbf{21.69 \%} & \textbf{-0.47 dB } \\
\hline
\end{tabular}
\caption{Measure of speedup and compression efficiency for intra-resolution analysis sharing with lowest QP (highest quality) representation as master/ base encode}
\label{tab:intra_resolution_result}
\end{table}

\begin{table}[!htbp]
\centering
\begin{tabular}{|p{2.8cm} | p{2.0cm} |p{2.5cm}| p{1.5cm}| p{1.5cm} |p{1.8cm} |}
\hline
\multicolumn{6}{|c|}{Test for CQP representations}\\
\hline
Video & Resolution & Analysis level &	$\Delta$T & BD-Rate & BD-PSNR\\
\hline
\rowcolor{blue!5} BasketBallDrive &	960x540 &	4 &	13.89 \% &	1.72 \% &	-0.08 dB \\
\rowcolor{gray!10} BasketBallDrive &	960x540 &	6 &	14.31 \% &	1.72 \% &	-0.08 dB \\
\rowcolor{blue!5} BasketBallDrive &	960x540 &	10 &	61.74 \% &	7.49 \% &	-0.34 dB \\
\rowcolor{gray!10} BasketBallDrive &	1920x1080 &	4 &	13.00 \% &	2.33 \% &	-0.05 dB \\
\rowcolor{blue!5} BasketBallDrive &	1920x1080 &	6 &	16.26 \% &	2.33 \% &	-0.05 dB \\
\rowcolor{gray!10} BasketBallDrive &	1920x1080 &	10 &	62.46 \% &	11.55 \% &	-0.26 dB \\
\rowcolor{blue!5} CrowdRun &	960x540 &	4 &	16.83 \% &	0.34 \% &	-0.01 dB \\
\rowcolor{gray!10} CrowdRun &	960x540 &	6 &	17.63 \% &	0.34 \% &	-0.01 dB \\
\rowcolor{blue!5} CrowdRun &	960x540 &	10 &	67.52 \% &	5.93 \% &	-0.22 dB \\
\rowcolor{gray!10} CrowdRun &	1920x1080 &	4 &	14.89 \% &	2.35 \% &	-0.09 dB \\
\rowcolor{blue!5} CrowdRun &	1920x1080 &	6 &	15.31 \% &	2.35 \% &	-0.09 dB \\
\rowcolor{gray!10} CrowdRun &	1920x1080 &	10 &	61.74 \% &	8.71 \% &	-0.32 dB \\
\rowcolor{blue!5} DucksTakeOff &	960x540 &	4 &	21.83 \% &	0.34 \% &	-0.01 dB \\
\rowcolor{gray!10} DucksTakeOff &	960x540 &	6 &	22.63 \% &	0.34 \%	 &-0.01 dB \\
\rowcolor{blue!5} DucksTakeOff &	960x540 &	10 &	67.52 \% &	5.93 \% &	-0.22 dB \\
\rowcolor{gray!10} DucksTakeOff &	1920x1080 &	4 &	13.83 \% &	0.14 \% &	0.00 dB \\
\rowcolor{blue!5} DucksTakeOff &	1920x1080 &	6 &	13.63 \% &	0.14 \% &	0.00 dB \\
\rowcolor{gray!10} DucksTakeOff &	1920x1080 &	10 &	67.52 \% &	5.51 \% &	-0.17 dB \\
\hline
\textbf{Average} & 960x540 & \textbf{4} &	 \textbf{16.94 \% }  &	\textbf{0.80 \%}  &	\textbf{-0.03 dB } \\
\textbf{Average} & 960x540 & \textbf{6} &	\textbf{18.77 \% }   &  \textbf{0.80 \%}  &	\textbf{-0.03 dB } \\
\textbf{Average} & 960x540 & \textbf{10} & \textbf{65.60 \% }&	\textbf{6.45 \%}   &	\textbf{-0.26 dB }\\
\hline
\textbf{Average} & 1920x1080 & \textbf{4} &	 \textbf{13.91 \% }  &	\textbf{1.61 \%} &  \textbf{-0.05 dB }\\
\textbf{Average} & 1920x1080 & \textbf{6} &	\textbf{15.07 \% }   &  \textbf{1.61 \%} &  \textbf{-0.05 dB }\\
\textbf{Average} & 1920x1080 & \textbf{10} & \textbf{63.91 \% } &	\textbf{8.59 \%} &	\textbf{-0.25 dB }\\
\hline
\end{tabular}
\caption{Measure of speedup and compression efficiency for intra-resolution analysis sharing with median QP representation as master/ base encode}
\label{tab:intra_resolution_median_result}
\end{table}

\begin{table}[!htbp]
\centering
\begin{tabular}{|p{2.8cm} | p{2.0cm} | p{2.0cm} | p{1.5cm}| p{1.5cm} |p{1.8cm} |}
\hline
\multicolumn{6}{|c|}{Test for CQP representations}\\
\hline
Video & Resolution & Refinement & $\Delta$T & BD-Rate & BD-PSNR\\
\hline
\rowcolor{gray!10} BasketBallDrive & 1920x1080 & no &	67.27 \% &	13.81 \% &	-0.29 dB \\
\rowcolor{blue!5} CrowdRun &	1920x1080 & no &	69.40 \% &	37.28 \% &	-1.22 dB\\
\rowcolor{gray!10} DucksTakeOff &	1920x1080 & no &	79.46 \% &	11.54 \% &	-0.34 dB\\
\hline
\textbf{Average} & 1920x1080 & no & \textbf{72.04 \% }  &	\textbf{20.08 \%}  & \textbf{-0.62 dB}\\
\hline
\rowcolor{gray!10} BasketBallDrive & 1920x1080 & yes &	31.99 \% &	-5.23 \% &	0.12 dB \\
\rowcolor{blue!5} CrowdRun &	1920x1080 & yes &	37.27 \% &	3.68 \% &	-0.14 dB\\
\rowcolor{gray!10} DucksTakeOff &	1920x1080 & yes &	17.72 \% &	6.37 \% &	-0.20 dB\\
\hline
\textbf{Average} & 1920x1080 & yes & \textbf{28.99 \% }  &	\textbf{1.61 \%}  & \textbf{-0.07 dB}\\
\hline
\end{tabular}
\caption{Measure of speedup and BD-rate for 1080p inter-resolution analysis sharing with 540p representation as the master/ base encode and analysis reuse level 10}
\label{tab:inter_resolution_1080p_result_detailed}
\end{table}
