# Supplementary material for: Multi-resolution encoding and optimization for next generation video compression
Source: arXiv:2301.12191 source file (2023-01-28)
Supplement: Supplementary file 2 [file _appendix.tex]

\appendix

%%%%%%%%%% DON'T DELETE THIS, REVERTS NUMBERING BACK %%%%%%%%%%%%%
\makeatletter
\renewcommand{\@makechapterhead}[1]{\vspace *{-10\p@ }{\parindent \z@ 
\raggedright \normalfont \ifnum \c@secnumdepth >\m@ne \Huge \bfseries 
\@chapapp \space \thechapter \vskip 10\p@ \fi #1\par \nobreak \vskip 30\p@ }}
\makeatother
%%%%%%%%%% DON'T DELETE THIS, REVERTS NUMBERING BACK %%%%%%%%%%%%%

\chapter{SSE4 SIMD optimizations}
\label{sec:sse4_test_res}
\begin{table}[]
\rowcolors{2}{gray!5}{gray!10}
\fontsize{8pt}{10pt}\selectfont
% [inline block 0: 23 envs, 101701 chars -> data_tex | \begin{tabular}{| p{3.8cm}| p{1.3cm}|  p{3.8cm}|  p{1.3cm}|  p{3.8cm}|  p{1.3cm}| } \hline...]

\end{table}
