# Supplementary material for: Multi-resolution encoding and optimization for next generation video compression
Source: arXiv:2301.12191 source file (2023-01-28)
Supplement: Supplementary file 4 [file kth_appendix2_sse4.tex]

\chapter{SSE4 SIMD optimization}
\label{sec:sse4_test_res}
\begin{table}
%\rowcolors{2}{gray!5}{gray!10}
\fontsize{8pt}{10pt}\selectfont
% [inline block 0: 8 envs, 57424 chars -> data_tex | \begin{tabular}{| p{3.3cm}| p{0.7cm}|  p{3.3cm}|  p{0.7cm}|  p{3.3cm}|  p{0.7cm}| } \hline...]

\end{table}
