# Supplementary material for: Multi-resolution encoding and optimization for next generation video compression
Source: arXiv:2301.12191 source file (2023-01-28)
Supplement: Supplementary file 5 [file kth_appendix3_avx2.tex]

\chapter{AVX2 SIMD optimization}
\label{sec:avx2_test_res}
\begin{table}
%\rowcolors{2}{gray!5}{gray!10}
\fontsize{8pt}{10pt}\selectfont
\begin{tabular}{| p{3.3cm}| p{0.7cm}|  p{3.3cm}|  p{0.7cm}|  p{3.3cm}|  p{0.7cm}| }
\hline
Primitive & IPC \newline Gain & Primitive & IPC \newline Gain & Primitive & IPC \newline Gain\\
\hline
                            dst4[2] & 1.02 &                    sad\_ac\_p[0][8x4] & 1.75 &                sad\_ac\_res[0][64x32] & 1.96\\
                            dst4[1] & 1.04 &                   sad\_ac\_p[0][16x4] & 1.77 &                 subtract\_res[32x64] & 1.97\\
                   sad\_ac\_p[1][8x2] & 1.22 &                sad\_ac\_res[1][64x16] & 1.77 &                sad\_ac\_res[1][32x32] & 1.99\\
              mean\_diff\_res[1][8x2] & 1.24 &                   sad\_ac\_p[0][32x4] & 1.79 &                 sad\_ac\_res[1][8x16] & 2\\
                sad\_ac\_res[1][16x2] & 1.26 &                   copy\_bipred[32x4] & 1.79 &                sad\_ac\_res[1][64x64] & 2\\
                 sad\_ac\_res[0][8x4] & 1.35 &                 subtract\_res[32x16] & 1.79 &                  subtract\_pix[32x8] & 2\\
                   sad\_ac\_p[0][8x2] & 1.4 &                 sad\_ac\_res[1][64x8] & 1.81 &                   sub\_weight[32x16] & 2\\
                  copy\_bipred[16x2] & 1.44 &                  subtract\_res[32x4] & 1.81 &                   sad\_ac\_p[1][16x8] & 2.02\\
                 sad\_ac\_res[1][8x2] & 1.48 &                   sad\_ac\_p[0][64x8] & 1.83 &                   sad\_ac\_p[0][8x16] & 2.03\\
                  sad\_ac\_p[1][16x2] & 1.49 &                    sad\_ac\_p[1][8x4] & 1.85 &                  sad\_ac\_p[0][32x32] & 2.04\\
                mean\_diff\_p[1][8x2] & 1.53 &                   sad\_ac\_p[1][32x8] & 1.85 &                  sad\_ac\_p[1][32x16] & 2.07\\
             mean\_diff\_res[1][16x2] & 1.56 &                 sad\_ac\_res[0][16x4] & 1.87 &                  subtract\_pix[64x8] & 2.07\\
                subtract\_pix[32x16] & 1.57 &                sad\_ac\_res[1][32x16] & 1.87 &                sad\_ac\_res[0][32x64] & 2.08\\
                subtract\_pix[64x16] & 1.58 &                  copy\_bipred[32x32] & 1.87 &                 subtract\_res[32x32] & 2.08\\     
                  sad\_ac\_p[1][32x4] & 1.59 &                 subtract\_pix[32x32] & 1.87 &                    sub\_weight[32x8] & 2.09\\
                 sad\_ac\_res[1][8x8] & 1.62 &                  subtract\_res[64x8] & 1.88 &                  sad\_ac\_p[0][64x16] & 2.11\\                
             \hline
\end{tabular}
\end{table}
\newpage
\begin{table}
%\rowcolors{2}{gray!5}{gray!10}
\fontsize{8pt}{10pt}\selectfont
\begin{tabular}{| p{3.3cm}| p{0.7cm}|  p{3.3cm}|  p{0.7cm}|  p{3.3cm}|  p{0.7cm}| }
\hline
Primitive & IPC \newline Gain & Primitive & IPC \newline Gain & Primitive & IPC \newline Gain\\
\hline
                  sad\_ac\_p[0][16x2] & 1.62 &                  sad\_ac\_res[0][8x2] & 1.91 &                  sad\_ac\_p[1][32x64] & 2.12\\
                  sad\_ac\_p[1][16x4] & 1.62 &                  sad\_ac\_res[1][8x4] & 1.91 &                  subtract\_res[32x8] & 2.12\\
                 sad\_ac\_p[0][32x64] & 1.62 &                   sad\_ac\_p[0][16x8] & 1.91 &                sad\_ac\_res[1][32x64] & 2.13\\
                 copy\_bipred[64x64] & 1.62 &                   sad\_ac\_p[1][64x8] & 1.91 &                   sub\_weight[64x32] & 2.13\\
                 subtract\_pix[32x4] & 1.62 &                sad\_ac\_res[1][64x32] & 1.91 &                 sad\_ac\_res[1][32x8] & 2.14\\
                 copy\_bipred[32x16] & 1.63 &                 subtract\_pix[32x64] & 1.91 &                   sub\_weight[64x16] & 2.14\\
                 sad\_ac\_p[1][64x64] & 1.65 &                sad\_ac\_res[1][16x16] & 1.92 &                 sad\_ac\_res[0][32x8] & 2.15\\
                   sub\_weight[32x4] & 1.67 &                 sad\_ac\_res[0][32x4] & 1.92 &                 sad\_ac\_res[0][8x32] & 2.17\\
                sad\_ac\_res[0][16x2] & 1.68 &                sad\_ac\_res[0][64x64] & 1.92 &                sad\_ac\_res[1][16x32] & 2.17\\
                 sad\_ac\_p[0][64x32] & 1.69 &                   sad\_ac\_p[1][8x32] & 1.93 &                  sad\_ac\_p[0][32x16] & 2.17\\
                 sad\_ac\_p[0][64x64] & 1.72 &                 sad\_ac\_res[0][8x16] & 1.94 &                 sad\_ac\_res[1][32x4] & 2.18\\
               mean\_diff\_p[1][16x2] & 1.74 &                sad\_ac\_res[0][16x64] & 1.94 &                 sad\_ac\_res[0][64x8] & 2.18\\
                sad\_ac\_res[1][16x4] & 1.74 &                   copy\_bipred[16x4] & 1.95 &                 subtract\_pix[64x64] & 2.18\\
                 copy\_bipred[64x16] & 1.74 &                  sad\_ac\_p[1][64x16] & 1.96 &                   sad\_ac\_p[0][8x32] & 2.19\\
                 sad\_ac\_p[1][64x32] & 2.19 &                   sad\_ac\_p[0][8x64] & 2.48 &                  subtract\_res[16x4] & 2.96\\
                  sub\_weight[32x64] & 2.19 &                  sad\_ac\_p[0][16x64] & 2.49 &                   sad\_ac\_p[0][32x8] & 2.98\\
                  sad\_ac\_p[1][8x16] & 2.21 &                  sad\_ac\_p[0][16x16] & 2.5 &                     calc\_sign[16x2] & 2.99\\
               sad\_ac\_res[0][16x16] & 2.21 &                    sub\_weight[16x4] & 2.5 &             mean\_diff\_res[1][16x32] & 3\\
               sad\_ac\_res[0][32x16] & 2.21 &                  subtract\_pix[16x2] & 2.52 &                   sub\_weight[16x16] & 3\\
                subtract\_pix[64x32] & 2.21 &                 mean\_diff\_p[1][8x4] & 2.53 &              mean\_diff\_res[0][16x2] & 3.03\\
                   sub\_weight[64x8] & 2.21 &                  subtract\_pix[16x4] & 2.53 &                    calc\_sign[32x32] & 3.06\\
                subtract\_res[64x64] & 2.22 &                 mean\_diff\_p[0][8x2] & 2.54 &              mean\_diff\_res[1][8x16] & 3.07\\
                       sad\_pp[16x2] & 2.23 &                   sad\_ac\_p[1][8x64] & 2.57 &               mean\_diff\_res[0][8x8] & 3.08\\
               sad\_ac\_res[0][32x32] & 2.23 &              mean\_diff\_res[1][16x4] & 2.57 &                 mean\_diff\_p[1][8x8] & 3.11\\
                sad\_ac\_res[1][16x8] & 2.25 &                 sad\_ac\_res[0][16x8] & 2.59 &                     calc\_sign[32x8] & 3.11\\
                 sad\_ac\_p[1][32x32] & 2.26 &                  sad\_ac\_p[1][16x32] & 2.59 &                struct\_ssd\_block\_s\_4 & 3.12\\
                 sad\_ac\_res[0][8x8] & 2.27 &                   copy\_bipred[32x8] & 2.61 &                     sad\_sp\_x3[16x8] & 3.14\\
                  sub\_weight[32x32] & 2.31 &                   sub\_weight[64x64] & 2.64 &                     calc\_sign[16x4] & 3.14\\
                  copy\_bipred[64x8] & 2.33 &                sad\_ac\_res[1][16x64] & 2.65 &                  copy\_bipred[16x16] & 3.17\\
                 subtract\_res[16x2] & 2.34 &                struct\_ssd\_block\_p\_4 & 2.65 &                mean\_diff\_p[0][16x2] & 3.2\\
                subtract\_res[64x32] & 2.34 &                    sad\_ac\_p[0][8x8] & 2.66 &                    sad\_sp\_x3[64x32] & 3.2\\
              mean\_diff\_res[0][8x2] & 2.37 &               mean\_diff\_res[1][8x4] & 2.68 &                     sad\_sp\_x4[16x4] & 3.21\\
                sad\_ac\_res[1][8x32] & 2.37 &                    sad\_sp\_x4[64x64] & 2.69 &              mean\_diff\_res[0][16x4] & 3.21\\
                subtract\_res[64x16] & 2.37 &               mean\_diff\_res[1][8x8] & 2.71 &                        sad\_pp[16x4] & 3.23\\
                    sad\_sp\_x4[16x2] & 2.38 &                  copy\_bipred[32x64] & 2.72 &                 subtract\_pix[16x64] & 3.24\\
                 sad\_ac\_p[1][16x16] & 2.38 &                 sad\_ac\_res[1][8x64] & 2.74 &                 subtract\_res[16x64] & 3.26\\
               sad\_ac\_res[0][64x16] & 2.38 &                    sad\_sp\_x4[32x64] & 2.75 &                    calc\_sign[64x16] & 3.3\\
                 copy\_bipred[64x32] & 2.38 &                 mean\_diff\_p[0][8x4] & 2.76 &                mean\_diff\_p[1][16x4] & 3.34\\
                 subtract\_pix[16x8] & 2.39 &                    calc\_sign[32x16] & 2.77 &                     sad\_sp\_x4[32x4] & 3.41\\
                    sad\_sp\_x3[16x2] & 2.4 &               mean\_diff\_res[0][8x4] & 2.79 &                mean\_diff\_p[1][8x16] & 3.42\\
                   sad\_ac\_p[1][8x8] & 2.41 &                 mean\_diff\_p[0][8x8] & 2.8 &                        sad\_sp[16x4] & 3.45\\
               sad\_ac\_res[0][16x32] & 2.41 &                   copy\_bipred[16x8] & 2.8 &              mean\_diff\_res[1][16x8] & 3.45\\
                 sad\_ac\_p[0][16x32] & 2.44 &                  sad\_ac\_p[1][16x64] & 2.83 &                mean\_diff\_p[0][16x8] & 3.47\\
                sad\_ac\_res[0][8x64] & 2.45 &                     calc\_sign[32x4] & 2.83 &                     sad\_sp\_x3[32x4] & 3.47\\
\hline
\end{tabular}
\end{table}
\newpage
\begin{table}
%\rowcolors{2}{gray!5}{gray!10}
\fontsize{8pt}{10pt}\selectfont
\begin{tabular}{| p{3.3cm}| p{0.7cm}|  p{3.3cm}|  p{0.7cm}|  p{3.3cm}|  p{0.7cm}| }
\hline
Primitive & IPC \newline Gain & Primitive & IPC \newline Gain & Primitive & IPC \newline Gain\\
\hline
                   sad\_sp\_x3[32x64] & 3.48 &             luma\_inv\_quant\_10b[8x4] & 3.84 &                mean\_diff\_p[0][8x16] & 4.19\\
                   sad\_sp\_x4[32x16] & 3.52 &              mean\_diff\_res[0][8x32] & 3.87 &                 subtract\_res[16x32] & 4.19\\
                  sub\_weight[16x32] & 3.53 &                     sad\_sp\_x4[64x8] & 3.88 &             mean\_diff\_res[1][64x16] & 4.2\\
              mean\_diff\_p[1][16x16] & 3.55 &                    block\_zero[64x8] & 3.9 &                mean\_diff\_p[0][8x32] & 4.22\\
                  sub\_weight[16x64] & 3.55 &              mean\_diff\_res[1][8x32] & 3.92 &                  copy\_bipred[16x64] & 4.23\\
                    sad\_sp\_x4[16x8] & 3.56 &              mean\_diff\_res[0][32x8] & 3.92 &                    sad\_sp\_x3[16x16] & 4.25\\
              mean\_diff\_p[0][64x16] & 3.57 &                    rdo\_clipmul[8x4] & 3.93 &                   block\_zero[64x64] & 4.29\\
                    sad\_sp\_x4[32x8] & 3.58 &                    calc\_sign[64x64] & 3.94 &                mean\_diff\_p[0][8x64] & 4.3\\
                subtract\_pix[16x16] & 3.59 &                    sub\_weight[16x8] & 3.97 &               mean\_diff\_p[1][64x32] & 4.31\\
                    sad\_sp\_x3[16x4] & 3.6 &                 ang\_fast\_copy[16x2] & 3.98 &             mean\_diff\_res[0][16x64] & 4.34\\
                subtract\_pix[16x32] & 3.61 &                   rdo\_clipmul[8x64] & 3.99 &              mean\_diff\_res[0][16x8] & 4.35\\
                   calc\_sign[32x64] & 3.61 &                     sad\_sp\_x3[64x8] & 4 &             mean\_diff\_res[0][64x64] & 4.35\\
             mean\_diff\_res[0][8x16] & 3.62 &             mean\_diff\_res[0][64x32] & 4 &               mean\_diff\_p[1][16x64] & 4.38\\
                    calc\_sign[16x8] & 3.63 &                  rdo\_clipmul[16x64] & 4 &                mean\_diff\_p[1][8x32] & 4.4\\
               mean\_diff\_p[1][16x8] & 3.65 &                        sad\_pp[32x4] & 4.02 &                  rdo\_clipmul[64x32] & 4.4\\
             mean\_diff\_res[1][32x4] & 3.67 &             mean\_diff\_res[1][16x16] & 4.03 &             mean\_diff\_res[0][32x64] & 4.41\\
                   sad\_sp\_x3[32x16] & 3.67 &              mean\_diff\_res[0][32x4] & 4.05 &                    rdo\_clipmul[8x8] & 4.41\\
               mean\_diff\_p[1][32x4] & 3.68 &                    sad\_sp\_x4[64x32] & 4.05 &               rdo\_num\_nonzero[16x2] & 4.42\\
                    calc\_sign[64x8] & 3.69 &                        sad\_pp[16x8] & 4.06 &                  copy\_bipred[16x32] & 4.43\\
            luma\_inv\_quant\_12b[8x4] & 3.7 &                    sad\_sp\_x4[32x32] & 4.06 &                       sad\_sp[64x32] & 4.44\\
                   sad\_sp\_x3[16x64] & 3.71 &               mean\_diff\_p[0][64x64] & 4.08 &             mean\_diff\_res[0][32x16] & 4.45\\
                 subtract\_res[16x8] & 3.71 &                    calc\_sign[16x32] & 4.08 &                  rdo\_clipmul[32x16] & 4.46\\
                   rdo\_clipmul[8x2] & 3.71 &                        sad\_sp[32x4] & 4.09 &                    sad\_sp\_x3[32x32] & 4.47\\
                   sad\_sp\_x4[16x64] & 3.75 &              mean\_diff\_res[1][8x64] & 4.11 &                        sad\_sp[32x8] & 4.49\\
                   calc\_sign[64x32] & 3.75 &                    sad\_sp\_x4[16x16] & 4.12 &                    sad\_sp\_x3[64x64] & 4.5\\
                   calc\_sign[16x64] & 3.76 &              mean\_diff\_res[1][32x8] & 4.12 &                mean\_diff\_p[1][32x8] & 4.51\\
                subtract\_res[16x16] & 3.77 &             mean\_diff\_res[0][16x16] & 4.13 &                   rdo\_clipmul[16x2] & 4.51\\
                   calc\_sign[16x16] & 3.78 &                     sad\_sp\_x3[32x8] & 4.16 &                   rdo\_clipmul[16x4] & 4.52\\
                      copy\_block[3] & 3.83 &              mean\_diff\_res[0][8x64] & 4.17 &                       sad\_pp[64x64] & 4.53\\
               mean\_diff\_p[0][16x4] & 3.84 &               mean\_diff\_p[1][64x64] & 4.18 &                   block\_zero[64x16] & 4.53\\
            mean\_diff\_res[1][32x16] & 4.57 &                  rdo\_clipmul[16x16] & 4.99 &                struct\_ssd\_block\_s\_8 & 5.7\\
              mean\_diff\_p[0][64x32] & 4.57 &               mean\_diff\_p[0][32x32] & 5.02 &            luma\_inv\_quant\_12b[16x8] & 5.7\\
            mean\_diff\_res[0][32x32] & 4.59 &               mean\_diff\_p[1][32x32] & 5.02 &                struct\_ssd\_block\_p\_8 & 5.72\\
                       sad\_sp[64x8] & 4.6 &                  rdo\_clipmul[64x16] & 5.02 &                 ang\_fast\_copy[64x8] & 5.72\\
                   sad\_sp\_x4[16x32] & 4.66 &              mean\_diff\_res[0][64x8] & 5.03 &                       sad\_sp[32x32] & 5.73\\
                   sad\_sp\_x3[64x16] & 4.66 &                  rdo\_clipmul[32x64] & 5.03 &                   rdo\_clipmul[8x32] & 5.76\\
               mean\_diff\_p[0][32x4] & 4.68 &               mean\_diff\_p[0][32x16] & 5.04 &                       sad\_pp[16x16] & 5.77\\
              mean\_diff\_p[0][16x64] & 4.7 &             luma\_inv\_quant\_10b[8x8] & 5.07 &                       satd\_pp[16x4] & 5.78\\
            luma\_inv\_quant\_12b[8x8] & 4.71 &                   rdo\_clipmul[8x16] & 5.08 &                       sad\_pp[32x32] & 5.79\\
               mean\_diff\_p[1][8x64] & 4.72 &                       sad\_sp[16x16] & 5.1 &                       sad\_sp[64x64] & 5.79\\
                      sad\_pp[64x32] & 4.72 &                  rdo\_clipmul[64x64] & 5.11 &               mean\_diff\_p[1][32x64] & 5.81\\
                  rdo\_clipmul[16x8] & 4.72 &                       sad\_sp[64x16] & 5.12 &               rdo\_num\_nonzero[16x4] & 6.02\\
               mean\_diff\_p[0][32x8] & 4.73 &              mean\_diff\_res[1][64x8] & 5.13 &             mean\_diff\_res[1][64x32] & 6.03\\
                       sad\_sp[16x2] & 4.74 &                      luma\_hpp\_12[0] & 5.14 &              rdo\_sign\_reapply[16x4] & 6.04\\
                   sad\_sp\_x3[16x32] & 4.75 &                      luma\_hpp\_10[0] & 5.17 &            luma\_inv\_quant\_10b[16x4] & 6.08\\
              mean\_diff\_p[0][16x32] & 4.75 &                        sad\_pp[64x8] & 5.2 &                       sad\_pp[32x64] & 6.16\\
                       sad\_pp[32x8] & 4.75 &               mean\_diff\_p[0][32x64] & 5.23 &                       sad\_sp[32x64] & 6.21\\
            mean\_diff\_res[0][64x16] & 4.75 &                mean\_diff\_p[1][64x8] & 5.33 &            luma\_inv\_quant\_12b[32x4] & 6.24\\
              mean\_diff\_p[0][16x16] & 4.76 &                        sad\_sp[16x8] & 5.37 &                       sad\_sp[16x32] & 6.31\\
            mean\_diff\_res[1][32x32] & 4.78 &            luma\_inv\_quant\_10b[8x16] & 5.37 &                ang\_fast\_copy[16x64] & 6.34\\
            mean\_diff\_res[1][32x64] & 4.82 &             mean\_diff\_res[0][16x32] & 5.44 &                       sad\_pp[16x32] & 6.35\\
                  block\_zero[64x32] & 4.83 &            luma\_inv\_quant\_12b[8x16] & 5.46 &                  rdo\_clipmul[32x32] & 6.37\\
              mean\_diff\_p[1][64x16] & 4.85 &                       sad\_pp[64x16] & 5.53 &                   luma\_vsp\_10[32x4] & 6.56\\
            mean\_diff\_res[1][16x64] & 4.89 &                       sad\_pp[32x16] & 5.54 &                    luma\_vss\_10[4x4] & 6.57\\
            mean\_diff\_res[1][64x64] & 4.9 &                   rdo\_clipmul[32x8] & 5.55 &                       copy\_block[4] & 6.71\\
              mean\_diff\_p[1][16x32] & 4.92 &                        ssd\_sp[16x2] & 5.62 &            luma\_inv\_quant\_12b[16x4] & 6.73\\
              mean\_diff\_p[1][32x16] & 4.94 &              rdo\_sign\_reapply[16x2] & 5.63 &                   add\_clip\_12[16x2] & 6.74\\
                   sad\_sp\_x4[64x16] & 4.95 &                    luma\_vsp\_12[4x4] & 5.67 &                    luma\_vss\_12[4x4] & 6.78\\
                  rdo\_clipmul[32x4] & 4.95 &                mean\_diff\_p[0][64x8] & 5.68 &                       sad\_pp[16x64] & 6.8\\
                 rdo\_clipmul[16x32] & 4.96 &                   rdo\_clipmul[64x8] & 5.69 &             rdo\_sign\_reapply[64x32] & 6.9\\
\hline
\end{tabular}
\end{table}
\newpage
\begin{table}
%\rowcolors{2}{gray!5}{gray!10}
\fontsize{8pt}{10pt}\selectfont
\begin{tabular}{| p{3.3cm}| p{0.7cm}|  p{3.3cm}|  p{0.7cm}|  p{3.3cm}|  p{0.7cm}| }
\hline
Primitive & IPC \newline Gain & Primitive & IPC \newline Gain & Primitive & IPC \newline Gain\\
\hline
           luma\_inv\_quant\_12b[8x32] & 6.95 &           luma\_inv\_quant\_12b[32x32] & 7.8 &            luma\_inv\_quant\_12b[8x64] & 8.4\\
           luma\_inv\_quant\_10b[8x32] & 6.97 &                    add\_avg\_12[16x2] & 7.84 &                       copy\_block[5] & 8.43\\
                       ssd\_sp[16x4] & 7 &                    luma\_vss\_10[8x4] & 7.84 &                    luma\_vss\_10[4x8] & 8.49\\
                   luma\_vps\_12[4x8] & 7 &                   luma\_vps\_10[4x16] & 7.87 &           luma\_inv\_quant\_12b[16x16] & 8.49\\
                       ssd\_pp[32x4] & 7.02 &                    luma\_vsp\_10[4x4] & 7.88 &           luma\_inv\_quant\_10b[32x16] & 8.51\\
                   luma\_vpp\_10[4x4] & 7.15 &           luma\_inv\_quant\_10b[64x64] & 7.93 &                 chroma\_vss\_12[16x2] & 8.64\\
                   luma\_vpp\_12[4x4] & 7.17 &                    add\_avg\_10[16x2] & 7.95 &           luma\_inv\_quant\_12b[16x64] & 8.65\\
                      satd\_pp[32x4] & 7.21 &                    luma\_vsp\_12[8x4] & 7.97 &           luma\_inv\_quant\_12b[32x16] & 8.66\\
                      sad\_sp[32x16] & 7.26 &                   block\_zero[32x16] & 7.98 &           luma\_inv\_quant\_10b[32x32] & 8.66\\
                   luma\_vsp\_10[4x8] & 7.32 &           luma\_inv\_quant\_10b[16x32] & 8.06 &           luma\_inv\_quant\_10b[16x64] & 8.69\\
                  luma\_vpp\_12[4x16] & 7.42 &                   luma\_vsp\_10[4x16] & 8.08 &           luma\_inv\_quant\_12b[16x32] & 8.71\\
                  luma\_vpp\_12[4x32] & 7.42 &           luma\_inv\_quant\_10b[64x32] & 8.09 &                 chroma\_vpp\_10[16x4] & 8.74\\
                   block\_zero[32x8] & 7.42 &                    luma\_vps\_10[8x4] & 8.11 &                   luma\_vss\_10[4x32] & 8.76\\
            rdo\_sign\_reapply[64x64] & 7.43 &                       satd\_pp[16x8] & 8.12 &             rdo\_sign\_reapply[64x16] & 8.84\\
                      satd\_pp[64x8] & 7.48 &              rdo\_sign\_reapply[32x4] & 8.12 &                      luma\_hpp\_12[1] & 8.88\\
           luma\_inv\_quant\_10b[16x8] & 7.48 &                   luma\_vsp\_12[4x16] & 8.13 &                      satd\_sp[64x16] & 8.91\\
                      satd\_pp[32x8] & 7.52 &                        ssd\_pp[16x2] & 8.14 &                    luma\_vss\_12[4x8] & 8.96\\
            rdo\_sign\_reapply[16x64] & 7.55 &             rdo\_sign\_reapply[32x32] & 8.14 &                    luma\_vss\_12[8x8] & 8.96\\
                  luma\_vss\_12[32x4] & 7.57 &                        ssd\_ss[16x2] & 8.15 &                    luma\_vsp\_12[4x8] & 8.98\\
                   chroma\_hps\_10[2] & 7.61 &                    luma\_vpp\_10[4x8] & 8.17 &                 chroma\_vss\_10[16x2] & 8.99\\
                      sad\_sp[16x64] & 7.65 &                        ssd\_pp[16x8] & 8.18 &           luma\_inv\_quant\_10b[64x16] & 9.01\\
                   block\_zero[32x4] & 7.65 &              rdo\_sign\_reapply[32x8] & 8.18 &                       satd\_sp[16x4] & 9.02\\
                  luma\_vsp\_12[16x4] & 7.71 &                 chroma\_vps\_10[16x2] & 8.23 &           luma\_inv\_quant\_10b[32x64] & 9.04\\
            rdo\_sign\_reapply[16x16] & 7.72 &                    chroma\_hps\_10[5] & 8.24 &              rdo\_sign\_reapply[16x8] & 9.04\\
                   luma\_vps\_12[4x4] & 7.74 &                       satd\_sp[32x4] & 8.25 &                ang\_fast\_copy[16x16] & 9.06\\
                  add\_clip\_10[16x2] & 7.75 &                  add\_clip\_12[16x32] & 8.34 &                    luma\_vss\_10[8x8] & 9.09\\
           luma\_inv\_quant\_10b[8x64] & 7.76 &             rdo\_sign\_reapply[32x64] & 8.34 &                   add\_clip\_10[16x4] & 9.09\\
           luma\_inv\_quant\_10b[64x8] & 7.77 &                      satd\_sp[32x64] & 8.35 &                  add\_clip\_10[16x64] & 9.1\\
                   luma\_vps\_10[4x8] & 7.79 &           luma\_inv\_quant\_10b[16x16] & 8.35 &                   block\_zero[32x64] & 9.11\\
                   luma\_vps\_10[4x4] & 7.8 &                    luma\_vpp\_12[8x4] & 8.4 &                   luma\_vsp\_10[8x16] & 9.13\\
                chroma\_vss\_10[32x4] & 9.15 &                 chroma\_vsp\_10[16x2] & 9.7 &                    luma\_vpp\_12[4x8] & 10.33\\
          luma\_inv\_quant\_12b[64x16] & 9.16 &            luma\_inv\_quant\_12b[64x8] & 9.73 &                   luma\_vps\_12[16x4] & 10.33\\
                  luma\_vss\_12[4x32] & 9.21 &                  luma\_vps\_12[16x64] & 9.75 &                   add\_clip\_10[16x8] & 10.33\\
                   luma\_vss\_12[8x4] & 9.22 &                 ang\_fast\_copy[16x4] & 9.75 &                   add\_clip\_12[64x8] & 10.38\\
                  luma\_vss\_12[4x16] & 9.23 &           luma\_inv\_quant\_12b[64x64] & 9.76 &                   luma\_vsp\_10[4x32] & 10.39\\
                  luma\_vpp\_12[16x8] & 9.23 &                      satd\_pp[32x32] & 9.79 &                       satd\_sp[32x8] & 10.4\\
          luma\_inv\_quant\_12b[32x64] & 9.24 &                      satd\_pp[32x16] & 9.81 &                   luma\_vss\_12[16x4] & 10.4\\
                  luma\_vps\_10[32x4] & 9.25 &                   luma\_vps\_10[16x4] & 9.81 &                chroma\_vpp\_10[64x32] & 10.41\\
                   luma\_vpp\_10[8x4] & 9.29 &                ang\_fast\_copy[32x64] & 9.81 &                   luma\_vpp\_12[32x4] & 10.44\\
                  luma\_vsp\_10[16x4] & 9.29 &                        ssd\_pp[16x4] & 9.89 &                      satd\_pp[16x64] & 10.46\\
                  luma\_vps\_10[4x32] & 9.3 &            luma\_inv\_quant\_10b[32x8] & 9.9 &                  luma\_vpp\_10[16x64] & 10.5\\
                   block\_zero[16x2] & 9.3 &             rdo\_sign\_reapply[32x16] & 9.92 &                      luma\_hpp\_10[1] & 10.51\\
          luma\_inv\_quant\_12b[64x32] & 9.3 &                   luma\_vpp\_10[4x32] & 9.97 &                   luma\_vpp\_12[32x8] & 10.52\\
                   add\_avg\_12[16x4] & 9.32 &                    luma\_vps\_10[8x8] & 9.97 &                   luma\_vss\_10[8x64] & 10.53\\
                  luma\_vps\_12[4x16] & 9.39 &                  luma\_vps\_12[32x32] & 10.01 &                   add\_avg\_10[32x16] & 10.61\\
               ang\_fast\_copy[16x32] & 9.39 &                  luma\_vps\_12[32x64] & 10.01 &                   luma\_vss\_10[8x16] & 10.61\\
               ang\_fast\_copy[32x32] & 9.39 &                  add\_clip\_12[16x64] & 10.1 &                   luma\_vpp\_12[16x4] & 10.61\\
                   add\_avg\_10[16x4] & 9.42 &                   luma\_vpp\_10[4x16] & 10.11 &                      luma\_hps\_10[1] & 10.65\\
                  luma\_vps\_12[4x32] & 9.43 &                    luma\_vps\_12[8x4] & 10.11 &                 ang\_fast\_copy[32x4] & 10.66\\
                  luma\_vsp\_10[16x8] & 9.44 &                 chroma\_vps\_10[16x4] & 10.12 &                      satd\_sp[64x64] & 10.67\\
                      satd\_sp[64x8] & 9.45 &                   luma\_vsp\_12[32x8] & 10.12 &                  luma\_vpp\_12[64x32] & 10.68\\
                  block\_zero[32x32] & 9.47 &                    luma\_vsp\_10[8x4] & 10.13 &                  luma\_vss\_10[16x64] & 10.7\\
                  luma\_vss\_10[4x16] & 9.51 &                  luma\_vsp\_12[32x32] & 10.13 &                   luma\_vpp\_10[16x4] & 10.75\\
              rdo\_num\_nonzero[32x4] & 9.51 &                ang\_fast\_copy[64x32] & 10.16 &                      satd\_sp[16x16] & 10.76\\
            rdo\_sign\_reapply[16x32] & 9.52 &                   luma\_vss\_10[32x8] & 10.21 &                  luma\_vsp\_10[64x16] & 10.81\\
                 luma\_vpp\_10[32x64] & 9.55 &              rdo\_num\_nonzero[16x16] & 10.23 &                 chroma\_vps\_10[32x4] & 10.85\\
             rdo\_sign\_reapply[64x8] & 9.55 &                   luma\_vss\_10[32x4] & 10.24 &                   luma\_vss\_10[16x4] & 10.85\\
           luma\_inv\_quant\_10b[32x4] & 9.59 &                   luma\_vpp\_10[32x4] & 10.27 &                   luma\_vpp\_10[16x8] & 10.85\\
                chroma\_vpp\_10[16x2] & 9.62 &                ang\_fast\_copy[32x16] & 10.3 &                      satd\_pp[16x16] & 10.89\\
                 add\_clip\_10[16x32] & 9.68 &                      satd\_pp[64x64] & 10.32 &                        ssd\_ss[16x4] & 10.9\\
\hline
\end{tabular}
\end{table}
\newpage
\begin{table}
%\rowcolors{2}{gray!5}{gray!10}
\fontsize{8pt}{10pt}\selectfont
\begin{tabular}{| p{3.3cm}| p{0.7cm}|  p{3.3cm}|  p{0.7cm}|  p{3.3cm}|  p{0.7cm}| }
\hline
Primitive & IPC \newline Gain & Primitive & IPC \newline Gain & Primitive & IPC \newline Gain\\
\hline
              rdo\_num\_nonzero[16x8] & 10.94 &                chroma\_vps\_10[32x32] & 11.58 &                        ssd\_ss[32x4] & 12.13\\
                     satd\_sp[32x16] & 11 &                 chroma\_vpp\_12[16x2] & 11.59 &                  luma\_vsp\_10[64x32] & 12.15\\
                   chroma\_hps\_10[3] & 11 &                      luma\_hps\_10[4] & 11.6 &                    luma\_vpp\_10[8x8] & 12.17\\
                 luma\_vsp\_10[16x64] & 11 &                chroma\_vsp\_10[32x16] & 11.63 &                  add\_clip\_10[16x16] & 12.21\\
               ang\_fast\_copy[64x16] & 11.01 &                  luma\_vsp\_12[16x64] & 11.64 &                chroma\_vss\_12[16x16] & 12.24\\
                       ssd\_sp[16x8] & 11.04 &                      satd\_pp[32x64] & 11.66 &                chroma\_vpp\_12[32x64] & 12.26\\
                     satd\_sp[16x32] & 11.04 &                  luma\_vps\_10[32x32] & 11.68 &                   luma\_vss\_12[8x32] & 12.27\\
                chroma\_vpp\_12[16x4] & 11.04 &                    luma\_vsp\_12[8x8] & 11.69 &                       ssd\_pp[32x32] & 12.28\\
                  luma\_vsp\_12[32x4] & 11.04 &                   luma\_vps\_10[8x32] & 11.71 &                  luma\_vpp\_12[32x64] & 12.28\\
                  luma\_vsp\_12[8x64] & 11.05 &                        ssd\_pp[32x8] & 11.72 &                    add\_avg\_12[16x8] & 12.3\\
        luma\_inv\_quant\_12b[32x8] & 11.05 &                 chroma\_vss\_12[16x4] & 11.75 &                 chroma\_vss\_10[16x4] & 12.33\\
                     satd\_pp[16x32] & 11.08 &                  luma\_vps\_12[16x32] & 11.75 &                    luma\_vsp\_10[8x8] & 12.38\\
                 luma\_vps\_10[32x64] & 11.08 &                  luma\_vps\_10[16x64] & 11.79 &                       ssd\_sp[64x16] & 12.48\\
                 luma\_vsp\_10[16x16] & 11.1 &               rdo\_num\_nonzero[32x8] & 11.8 &                  luma\_vps\_12[64x64] & 12.5\\
               ang\_fast\_copy[64x64] & 11.1 &               rdo\_num\_nonzero[64x8] & 11.8 &                chroma\_vsp\_10[16x32] & 12.51\\
                     satd\_pp[64x32] & 11.17 &                   luma\_vps\_12[32x4] & 11.81 &                  luma\_vss\_12[16x64] & 12.51\\
               chroma\_vpp\_12[64x16] & 11.17 &                    add\_avg\_10[16x8] & 11.82 &                        ssd\_sp[32x4] & 12.53\\
                     satd\_pp[64x16] & 11.18 &                 chroma\_vsp\_10[16x4] & 11.82 &                 chroma\_vpp\_12[32x8] & 12.53\\
               chroma\_vpp\_12[64x32] & 11.2 &                   luma\_vps\_12[32x8] & 11.82 &                   block\_zero[16x32] & 12.53\\
                  add\_clip\_12[16x4] & 11.2 &                   block\_zero[16x16] & 11.85 &                   luma\_vss\_12[32x8] & 12.55\\
                      satd\_sp[16x8] & 11.23 &                  luma\_vss\_12[16x16] & 11.87 &                      satd\_sp[16x64] & 12.58\\
                 luma\_vps\_10[64x32] & 11.3 &                  luma\_vss\_12[64x64] & 11.88 &                   luma\_vss\_10[64x8] & 12.58\\
                 luma\_vps\_10[64x64] & 11.35 &                   luma\_vss\_12[8x64] & 11.89 &                chroma\_vpp\_12[16x16] & 12.64\\
                 luma\_vss\_12[32x16] & 11.42 &                chroma\_vpp\_10[32x64] & 11.9 &                  add\_clip\_12[32x16] & 12.64\\
                  luma\_vsp\_12[4x32] & 11.43 &                  add\_clip\_12[16x16] & 11.91 &                 chroma\_vsp\_10[32x4] & 12.68\\
                  luma\_vsp\_12[16x8] & 11.44 &                    add\_avg\_12[32x4] & 11.92 &                chroma\_vpp\_10[16x64] & 12.69\\
                  add\_clip\_12[16x8] & 11.47 &                   luma\_vss\_12[8x16] & 11.93 &                   luma\_vss\_12[16x8] & 12.72\\
                   chroma\_hps\_10[4] & 11.48 &                   luma\_vss\_10[16x8] & 11.93 &                 chroma\_vss\_12[32x4] & 12.73\\
                 add\_clip\_10[64x16] & 11.48 &                chroma\_vps\_10[64x16] & 11.95 &                  luma\_vpp\_12[16x16] & 12.74\\
                  add\_clip\_10[32x4] & 11.52 &                  add\_clip\_12[64x32] & 12.1 &                   luma\_vps\_12[8x32] & 12.78\\
                 luma\_vss\_10[32x16] & 12.8 &                  luma\_vps\_12[64x32] & 13.27 &                  luma\_vps\_12[16x16] & 13.76\\
                     satd\_sp[64x32] & 12.81 &                      luma\_hpp\_12[3] & 13.3 &                   luma\_vps\_12[16x8] & 13.78\\
                     luma\_hpp\_12[2] & 12.82 &                chroma\_vsp\_10[32x32] & 13.31 &                  luma\_vsp\_10[32x16] & 13.81\\
                 luma\_vss\_12[16x32] & 12.83 &                   luma\_vps\_10[32x8] & 13.31 &                   add\_avg\_10[16x64] & 13.84\\
               chroma\_vps\_10[16x64] & 12.84 &                  luma\_vss\_10[32x64] & 13.31 &                 chroma\_vpp\_12[32x4] & 13.84\\
                 add\_clip\_10[32x64] & 12.84 &                    luma\_vpp\_12[8x8] & 13.32 &                  luma\_vss\_12[64x32] & 13.84\\
                ang\_fast\_copy[16x8] & 12.86 &                      satd\_sp[32x32] & 13.34 &                       ssd\_pp[16x32] & 13.87\\
               chroma\_vsp\_10[32x64] & 12.87 &                   luma\_vps\_10[8x16] & 13.37 &                  luma\_vsp\_12[16x32] & 13.87\\
                 add\_clip\_12[32x32] & 12.87 &                  luma\_vss\_10[64x16] & 13.37 &                  luma\_vss\_10[64x64] & 13.91\\
                  add\_avg\_12[16x32] & 12.89 &                   luma\_vps\_12[8x64] & 13.41 &                   luma\_vsp\_10[32x8] & 13.94\\
                  add\_avg\_12[64x64] & 12.93 &                  luma\_vss\_10[64x32] & 13.41 &                   luma\_vsp\_10[64x8] & 13.94\\
               chroma\_vss\_10[16x16] & 12.95 &                chroma\_vss\_12[64x64] & 13.43 &                 chroma\_vsp\_10[16x8] & 13.95\\
                chroma\_vss\_12[64x8] & 12.97 &              rdo\_num\_nonzero[16x32] & 13.44 &                   luma\_vss\_12[64x8] & 13.95\\
                       ssd\_sp[32x8] & 12.98 &                chroma\_vss\_10[64x64] & 13.46 &                 chroma\_vpp\_12[16x8] & 14.01\\
                  add\_clip\_12[32x4] & 12.98 &                  luma\_vpp\_12[16x32] & 13.46 &                  luma\_vpp\_12[32x32] & 14.01\\
                 luma\_vss\_10[16x32] & 13 &                chroma\_vss\_12[64x32] & 13.47 &                 chroma\_vsp\_10[32x8] & 14.07\\
                 luma\_vps\_10[16x16] & 13.03 &                  luma\_vpp\_10[32x32] & 13.49 &                   luma\_vsp\_10[8x32] & 14.09\\
                   luma\_vps\_12[8x8] & 13.04 &                  luma\_vss\_12[32x32] & 13.52 &                  luma\_vsp\_12[16x16] & 14.09\\
               chroma\_vpp\_10[64x64] & 13.05 &                   block\_zero[16x64] & 13.56 &                   add\_clip\_10[32x8] & 14.1\\
                 luma\_vss\_12[64x16] & 13.05 &                   luma\_vss\_10[8x32] & 13.57 &                       ssd\_pp[64x64] & 14.16\\
                  luma\_vsp\_12[8x16] & 13.07 &                   luma\_vps\_10[16x8] & 13.61 &                 chroma\_vpp\_10[16x8] & 14.19\\
                 luma\_vss\_10[16x16] & 13.1 &                  luma\_vps\_12[32x16] & 13.62 &                chroma\_vpp\_10[32x16] & 14.2\\
                  luma\_vpp\_10[64x8] & 13.13 &                    block\_zero[16x8] & 13.63 &                       ssd\_pp[32x16] & 14.21\\
                       ssd\_ss[16x8] & 13.14 &                  luma\_vsp\_10[32x32] & 13.64 &                chroma\_vps\_10[16x32] & 14.23\\
                   add\_avg\_10[32x4] & 13.14 &                   luma\_vpp\_12[8x16] & 13.65 &                   luma\_vsp\_12[8x32] & 14.23\\
                     luma\_hpp\_10[2] & 13.15 &                 ang\_fast\_copy[32x8] & 13.68 &                  luma\_vps\_12[64x16] & 14.25\\
                 add\_clip\_10[32x32] & 13.22 &                chroma\_vsp\_10[64x64] & 13.69 &                       ssd\_ss[32x16] & 14.26\\
               chroma\_vsp\_10[16x64] & 13.24 &                chroma\_vsp\_10[16x16] & 13.72 &                  luma\_vpp\_10[64x16] & 14.33\\
                 luma\_vps\_10[32x16] & 13.26 &                 chroma\_vss\_10[16x8] & 13.73 &                chroma\_vss\_10[64x16] & 14.34\\
               chroma\_vps\_10[64x64] & 13.27 &                   luma\_vps\_10[8x64] & 13.74 &                   luma\_vpp\_10[8x32] & 14.35\\
\hline
\end{tabular}
\end{table}
\newpage
\begin{table}
%\rowcolors{2}{gray!5}{gray!10}
\fontsize{8pt}{10pt}\selectfont
\begin{tabular}{| p{3.3cm}| p{0.7cm}|  p{3.3cm}|  p{0.7cm}|  p{3.3cm}|  p{0.7cm}| }
\hline
Primitive & IPC \newline Gain & Primitive & IPC \newline Gain & Primitive & IPC \newline Gain\\
\hline
                 luma\_vsp\_12[64x32] & 14.35 &                   luma\_vpp\_10[32x8] & 14.98 &                  add\_clip\_10[64x64] & 15.52\\
                       ssd\_ss[32x8] & 14.41 &                      luma\_hps\_10[3] & 15.01 &                   add\_clip\_12[32x8] & 15.54\\
                 luma\_vpp\_10[16x16] & 14.43 &                      luma\_hpp\_10[4] & 15.01 &                       ssd\_ss[32x32] & 15.56\\
                      ssd\_sp[32x16] & 14.44 &                 chroma\_vps\_10[32x8] & 15.02 &                chroma\_vps\_10[16x16] & 15.56\\
                chroma\_vps\_10[16x8] & 14.44 &                   add\_clip\_10[64x8] & 15.07 &                chroma\_vss\_10[32x16] & 15.58\\
                chroma\_vpp\_10[32x4] & 14.45 &                chroma\_vpp\_12[32x32] & 15.09 &                chroma\_vss\_12[32x64] & 15.58\\
                  luma\_vpp\_12[8x32] & 14.49 &                  luma\_vsp\_12[64x64] & 15.09 &                chroma\_vpp\_12[32x16] & 15.59\\
                 luma\_vps\_10[64x16] & 14.55 &                chroma\_vss\_12[32x32] & 15.1 &                chroma\_vsp\_10[64x16] & 15.59\\
                   add\_avg\_12[32x8] & 14.56 &                chroma\_vps\_10[32x16] & 15.13 &                       ssd\_sp[32x32] & 15.61\\
                     luma\_hpp\_10[3] & 14.59 &                       ssd\_sp[16x16] & 15.16 &                      luma\_hpp\_12[4] & 15.66\\
                chroma\_vss\_10[32x8] & 14.6 &                      luma\_hps\_10[2] & 15.16 &                       ssd\_ss[64x32] & 15.68\\
                  add\_avg\_12[16x16] & 14.61 &                   luma\_vpp\_10[8x16] & 15.18 &                chroma\_vsp\_10[64x32] & 15.68\\
                      ssd\_pp[16x16] & 14.66 &                chroma\_vss\_10[32x64] & 15.19 &                  luma\_vpp\_10[32x16] & 15.7\\
                  add\_avg\_12[32x32] & 14.66 &                chroma\_vss\_12[64x16] & 15.24 &                 chroma\_vpp\_10[32x8] & 15.72\\
                  luma\_vsp\_12[64x8] & 14.66 &                chroma\_vps\_10[32x64] & 15.27 &                       ssd\_sp[64x32] & 15.75\\
                chroma\_vss\_12[16x8] & 14.7 &                  luma\_vsp\_10[32x64] & 15.29 &              rdo\_num\_nonzero[16x64] & 15.77\\
                 add\_clip\_12[32x64] & 14.71 &                       ssd\_ss[64x16] & 15.33 &                 chroma\_vps\_10[64x8] & 15.83\\
                 luma\_vsp\_12[32x16] & 14.72 &                chroma\_vpp\_10[16x32] & 15.33 &                   add\_avg\_10[32x32] & 15.86\\
                  luma\_vps\_10[64x8] & 14.74 &                       ssd\_ss[16x16] & 15.38 &              rdo\_num\_nonzero[32x16] & 15.89\\
                 luma\_vpp\_12[64x16] & 14.74 &                        ssd\_sp[64x8] & 15.39 &                 chroma\_vss\_10[64x8] & 15.94\\
               chroma\_vss\_10[64x32] & 14.75 &                       ssd\_pp[64x16] & 15.39 &                  luma\_vpp\_10[16x32] & 15.94\\
               chroma\_vpp\_12[64x64] & 14.76 &                  luma\_vpp\_10[64x64] & 15.39 &                  luma\_vsp\_12[64x16] & 15.94\\
                 luma\_vpp\_12[32x16] & 14.8 &                  luma\_vsp\_10[16x32] & 15.4 &                chroma\_vpp\_10[32x32] & 16.05\\
               chroma\_vpp\_12[16x64] & 14.84 &                   add\_avg\_12[32x16] & 15.41 &                  add\_clip\_12[64x64] & 16.12\\
                  luma\_vpp\_10[8x64] & 14.87 &                   add\_avg\_10[16x16] & 15.43 &                   add\_avg\_12[16x64] & 16.14\\
                 luma\_vps\_10[16x32] & 14.89 &                 chroma\_vss\_12[32x8] & 15.44 &                       ssd\_pp[64x32] & 16.27\\
                  luma\_vps\_12[64x8] & 14.91 &                chroma\_vpp\_10[64x16] & 15.44 &                       ssd\_sp[32x64] & 16.35\\
                chroma\_vpp\_10[64x8] & 14.97 &                 chroma\_vsp\_10[64x8] & 15.5 &                        ssd\_pp[64x8] & 16.38\\
                chroma\_vpp\_12[64x8] & 14.97 &                chroma\_vpp\_10[16x16] & 15.52 &                   add\_avg\_10[16x32] & 16.42\\
                 add\_clip\_10[32x16] & 14.97 &                  add\_clip\_12[64x16] & 15.52 &                  luma\_vss\_10[32x32] & 16.48\\
                 luma\_vsp\_12[32x64] & 16.57 &                       ssd\_sp[16x64] & 17.14 &              rdo\_num\_nonzero[64x32] & 17.96\\
               chroma\_vss\_10[32x32] & 16.58 &                       ssd\_pp[16x64] & 17.21 &                chroma\_vss\_12[16x64] & 18.43\\
                      ssd\_sp[16x32] & 16.66 &                   luma\_vsp\_10[8x64] & 17.23 &                    add\_avg\_12[64x8] & 18.44\\
                   add\_avg\_10[32x8] & 16.68 &                   add\_avg\_12[64x16] & 17.25 &                chroma\_vps\_10[64x32] & 18.49\\
               chroma\_vpp\_12[16x32] & 16.73 &                       ssd\_ss[16x64] & 17.31 &                   add\_avg\_10[64x64] & 19.13\\
               chroma\_vss\_12[32x16] & 16.75 &              rdo\_num\_nonzero[64x16] & 17.44 &                chroma\_vss\_10[16x32] & 19.2\\
                      ssd\_pp[32x64] & 16.83 &                    add\_avg\_10[64x8] & 17.51 &              rdo\_num\_nonzero[32x64] & 19.28\\
                 luma\_vss\_12[32x64] & 16.84 &                   luma\_vpp\_12[8x64] & 17.57 &                   add\_avg\_10[64x32] & 19.31\\
                  luma\_vpp\_12[64x8] & 16.92 &                  luma\_vsp\_10[64x64] & 17.59 &                  luma\_vpp\_12[16x64] & 19.67\\
                  add\_avg\_10[32x64] & 16.97 &              rdo\_num\_nonzero[32x32] & 17.62 &                    block\_zero[16x4] & 19.78\\
                 add\_clip\_10[64x32] & 16.98 &                  luma\_vpp\_12[64x64] & 17.71 &                       ssd\_ss[16x32] & 19.84\\
                  luma\_vps\_12[8x16] & 17.02 &                   add\_avg\_12[32x64] & 17.91 &              rdo\_num\_nonzero[64x64] & 19.85\\
               chroma\_vss\_12[16x32] & 17.05 &                chroma\_vss\_10[16x64] & 17.94 &                       ssd\_ss[32x64] & 21.72\\
                  add\_avg\_12[64x32] & 17.11 &                   add\_avg\_10[64x16] & 17.96 &                  luma\_vpp\_10[64x32] & 22.48\\
                       ssd\_ss[64x8] & 23.33 &  &  &  & \\
\hline
\end{tabular}
\end{table}
